# Supplementary material for: Visual Concept Networks: A Graph-Based Approach to Detecting Anomalous Data in Deep Neural Networks
Source: arXiv:2409.18235 source file (2024-09-26)
Supplement: Supplementary file 1 [file appendix.tex]

\begin{figure*}[!t]  % The 't' flag tries to place the content at the top of the page
\section{Imagenet Data Construction}

\noindent The ImageNet structure, once accessible at \url{https://image-net.org/api/xml/structure_released.xml}, is no longer available and is now an archived resource to be shared later. ImageNet's categories, termed as synsets, are derived from WordNet's hierarchical framework. WordNet is an English lexical database where words are grouped into synsets based on their cognitive synonyms, all interwoven through semantic and lexical connections. ImageNet aimed to represent each WordNet synset with around 1000 images. However, not every synset has images in ImageNet. In the parsed tree structure of ImageNet, only top-tier synsets were chosen for individual distribution, and classes with fewer than 100 images were excluded.

The data and code necessary to replicate our results will be made available upon the paper's acceptance, with the exception of ImageNet due to its licensing constraints. Additionally, we have included several high-level algorithmic sketches of the experimental procedure to aid readers in grasping the intricacies of our experiment.
\end{figure*}

\begin{algorithm*}
\caption{Creation of Graph with Edge Weighting based on Distance and IoU}
\begin{algorithmic}[1]

\Procedure{create\_graph}{unique, temp, temp\_points}
    \State $G \gets$ Initialize empty graph
    \State Add nodes from 0 to length(unique) to $G$
    
    \If{length(temp) $> 1$}
        \State edges $\gets$ combinations of temp taken 2 at a time
        \State edgepoints $\gets$ combinations of temp\_points taken 2 at a time

        \For{$i$ from 0 to length(edges)}
            \State e $\gets$ edges[$i$]
            \State e\_wt $\gets$ edgepoints[$i$]
            
            \State Add edge between unique.index(e[0]) and unique.index(e[1]) to $G$
            \State Assign weight as $1 + \text{find\_distance}(e\_wt[0], e\_wt[1]) \times \text{find\_IoU}(e\_wt[0], e\_wt[1])$
        \EndFor
    \EndIf
    
    \State \Return G
\EndProcedure

\Procedure{find\_distance}{a, b}
    \State \Return $\sqrt{(a[0] - b[0])^2 + (a[1] - b[1])^2}$
\EndProcedure

\Procedure{find\_IoU}{a, b}
    \State $xA \gets \max(a[0], b[0])$
    \State $yA \gets \max(a[1], b[1])$
    \State $xB \gets \min(a[2], b[2])$
    \State $yB \gets \min(a[3], b[3])$

    \State inter\_area $\gets \max(0, xB - xA + 1) \times \max(0, yB - yA + 1)$
    \State a\_area $\gets (a[2] - a[0] + 1) \times (a[3] - a[1] + 1)$
    \State b\_area $\gets (b[2] - b[0] + 1) \times (b[3] - b[1] + 1)$

    \State \Return $\frac{\text{inter\_area}}{a\_area + b\_area - \text{inter\_area}}$
\EndProcedure

\end{algorithmic}
\end{algorithm*}

\begin{algorithm*}[!h]
\caption{Embedding and Classification of Graphs}
\begin{algorithmic}[1]

\Procedure{main}{}
    \State $\text{Initialize X, y, unique, unique\_index}$
    
    \For{file\_path, class\_label \textbf{in} json\_locations, class\_labels}
        \State $\text{results\_list} \gets \text{process\_results(file\_path)}$
        
        \For{results \textbf{in} results\_list}
            \State $\text{objects, object\_locations} \gets \text{filter\_results(results, CONFIDENCE\_THRESHOLD)}$
            \State $G \gets \text{create\_graph(unique\_class\_indexes, objects, object\_locations)}$
            \State $\text{Append G to X and class\_label to y}$
        \EndFor
    \EndFor
    
    \State $\text{X\_train, X\_test, y\_train, y\_test} \gets \text{train\_test\_split(X, y)}$

    \For{embedder\_name \textbf{in} embedders}
        \State $\text{embedder} \gets \text{initialize\_embedder(embedder\_name)}$
        \State $\text{Fit embedder on X\_train to get X\_train\_embedded}$
        \State $\text{Infer using embedder on X\_test to get X\_test\_embedded}$

        \For{classifier \textbf{in} classifiers}
            \State $\text{Train classifier on X\_train\_embedded and evaluate on X\_test\_embedded}$
            \State $\text{Print results}$
        \EndFor
    \EndFor
\EndProcedure

\Procedure{get\_unique\_classes}{vocabulary\_name}
    \State \text{Load vocabulary file based on vocabulary\_name}
    \State \text{Return unique classes}
\EndProcedure

\Procedure{process\_results}{file\_path}
    \State \text{Read JSON objects from file\_path}
    \State \text{Extract names, boxes, scores and map image\_path to these details}
    \State \text{Return results list}
\EndProcedure

\end{algorithmic}
\end{algorithm*}

\begin{algorithm*}
\caption{Generate Third-to-Top Level Synset Mapping on ImageNet}
\begin{algorithmic}[1]
\Procedure{GetSynsetMapping}{$xml\_filepath$}
    \State $tree \gets$ parse($xml\_filepath$)
    \State $synset\_map \gets$ empty dictionary
    
    \For{each $synset$ in $tree$.\textbf{iter}('synset')}
        \State $wnid \gets synset$.\textbf{attrib}['wnid']
        \State $ancestors \gets$ list($synset$.\textbf{iterancestors}())
        
        \If{length($ancestors$) $\geq$ 3}
            \State $synset\_map[wnid] \gets ancestors[-3]$.\textbf{attrib}['wnid']
        \Else
            \State $synset\_map[wnid] \gets wnid$
        \EndIf
    \EndFor
    
    \State \Return $synset\_map$
\EndProcedure

\text{We use the 3rd to top-level because of the structure of ImageNet XML. These are the equivalent of the top level.}
\end{algorithmic}
\end{algorithm*}

\begin{algorithm*}
\caption{Graph Embeddings and One-Class SVM Classification}
\begin{algorithmic}[1]
\Procedure{Main}{}
    \State \textbf{parse} command-line arguments for class names, file paths, threshold, and vocabulary
    \State \textbf{define} vocabulary mapping to different datasets
    
    \For{each given class}
        \State \textbf{load} JSON results for each class
        \State \textbf{process} each JSON entry to extract bounding box, object names, and scores
        \State \textbf{create} a graph based on the extracted results
        \State \textbf{store} graphs and their labels
    \EndFor
    
    \State \textbf{initialize} set of graph embedders and classifiers
    
    \For{each embedder}
        \State \textbf{fit} embedder on the training data
        \State \textbf{infer} embeddings for evaluation data
        \State \textbf{initialize} One-Class SVM and \textbf{train} on class\_1 embeddings
        \State \textbf{predict} on training and evaluation data
        \State \textbf{compute} AUC and accuracy metrics for the predictions
        \State \textbf{save} embeddings to a file for future use
    \EndFor
\EndProcedure
\end{algorithmic}
\end{algorithm*}

\begin{algorithm*}
\caption{Mahalanobis Distance for In-Distribution and Out-of-Distribution Detection}
\begin{algorithmic}[1]
\Procedure{Main}{}
    \State $(\text{labels}, \text{embeddings}) \gets \text{load\_embeddings\_from\_file}(\text{filename})$
    \State \text{split} $\text{embeddings}$ \text{into} \text{in\_dist} \text{and} \text{out\_dist} \text{based on labels}
    \State $\text{mean\_in} \gets \text{np.mean(in\_dist, axis=0)}$
    \State $\text{cov\_in} \gets \text{np.cov(in\_dist, rowvar=False)}$
    \State $\text{mahal\_in\_dist} \gets \text{mahalanobis\_distance\_efficient(in\_dist, mean\_in, cov\_in)}$
    \State $\text{mahal\_out\_dist} \gets \text{mahalanobis\_distance\_efficient(out\_dist, mean\_in, cov\_in)}$
    \State \text{Compute ROC and AUC} 
    \State \text{Compute Precision-Recall and AUCPR}
\EndProcedure

\Procedure{mahalanobis\_distance\_efficient}{$x$, $\text{mean}$, $\text{cov\_matrix}$}
    \State $x\_minus\_mu \gets x - \text{mean}$
    \State $\text{left\_term} \gets \text{solve(cov\_matrix, } x\_minus\_mu^T)^T$
    \State $\text{mahal} \gets \text{np.sum(} x\_minus\_mu \times \text{left\_term}, \text{axis=1)}$
    \Return mahal
\EndProcedure

\Procedure{load\_embeddings\_from\_file}{$\text{filename}$}
    \State \text{Read} $\text{filename}$ \text{and extract} $\text{labels}$ \text{and} $\text{embeddings}$
    \Return labels, embeddings
\EndProcedure
\end{algorithmic}
\end{algorithm*}
